# Supplementary material for: Multiple Query Optimization using a Hybrid Approach of Classical and Quantum Computing
Source: arXiv:2107.10508 source file (2021-07-22)
Supplement: Supplementary file 1 [file appendix.tex]

\onecolumn\newpage
\appendix

\section{First section of the appendix}
Quantum allows the usage of appendices.

\subsection{Subsection}
Ideally, the command \texttt{\textbackslash{}appendix} should be put before the appendices to get appropriate section numbering.
The appendices are then numbered alphabetically, with numeric (sub)subsection numbering.
Equations continue to be numbered sequentially.
\begin{equation}
  A \neq B
\end{equation}
You are free to change this in case it is more appropriate for your article, but a consistent and unambiguous numbering of sections and equations must be ensured.

If you want your appendices to appear in \texttt{onecolumn} mode but the rest of the document in \texttt{twocolumn} mode, you can insert the command \texttt{\textbackslash{}onecolumn\textbackslash{}newpage} before \texttt{\textbackslash{}appendix}.
